# Supplementary material for: What Makes and Breaks Safety Fine-tuning? A Mechanistic Study
Source: arXiv:2407.10264 source file (2024-08-21)
Supplement: Supplementary file 1 [file C.AnalyticalLipschitz.tex]

\section{Analytical Analysis of Lipschitz Constant}
\label{sec:lips_analytical_analysis}
Consider a single layer pre-trained neural network ${f:~} \mathbb{R^{d}}\xrightarrow{}\mathbb{R^{k}}$ with weight ${W}$ ($\mathbb{R^{d\times k}}$), given by  ${{f}(x,y) = W^Tx}$, where ${k}$ is the number of classes. We consider the following assumptions:
\begin{itemize}
    \item \textbf{A1:} Let all the fine-tuning samples $x$ in the set {${P}$} = \safepr $\cup$ \unsafepr be orthonormal to each other ie. ${x_i^Tx_j=0}$ $\forall {i,j}; {i\neq j}$ and ${x_i^Tx_i=1}$.
    \item \textbf{A2:} Let the weights of the pre-trained model given by ${{W^T[c]=\Sigma_{i=1}^{n_c}\delta_ix_{i,c}}}$, where ${\delta_i}\geq0$, ${n_c}$ is the number of samples belonging to class ${c}$ and used for pre-training. Therefore, such a model gives perfect classification performance on samples used during pre-training.
    \item \textbf{A3:} Let the fine-tuning setting be defined as a single token prediction, where for unsafe samples, the model needs to predict the null token and for the safe samples, the model should predict any one of the remaining ${r-1}$ classes, where ${r}$ is the total number of classes. Let the class index corresponding to null token prediction be 1.
\end{itemize}

\subsection{Analysis of global lipschitzness}
The global lipschitzness constant of a function ${f}$ on a set $\mathcal{P}$ is defined as \citep{sanyal2019stable}:
\begin{equation}
\label{eq:lips}
   {L({f})} =  {max_{x_i, x_j} \frac{||{f}(x_i) - {f}({x_j})||_q}{||{x_i}-{x_j}||_p}}
\end{equation}
where, ${x_i}, {x_j}$ are any two different samples ie. ${i \neq j}$ drawn from $\mathcal{P}$. Let ${p=q=2}$.
Let the safety fine-tuning learning rate be given by $\alpha$ and the hyperparameter used in DPO  and unlearning be 1. For simplicity, in this analysis we use the same hyperparameter value for the positive and negative terms in DPO and unlearning. Thus we have
\begin{prop}
\label{prop:Unlearning} $\exists$ learning rate ${\alpha}$ where ${\alpha}<min({\delta_i})$, $\forall {i\leq n_c, \forall c\leq r}$  such that $\forall$ input samples  ${x} \in  \bgdbox{red}{$\mathcal{P_U}$}$, we have
${L({f_{\theta^{Unl}}})} \leq {L({f_{\theta^{SSFT}}})} \leq {L({f_{\theta^{IT}}})}$
\end{prop}
\begin{proof}
 Let ${x}$ be the input sample sampled from either \bgdbox{green}{$\mathcal{P_S}$} or  \bgdbox{red}{$\mathcal{P_U}$} and ${y_L}$, ${y_P}$ be the less preferred and more preferred output labels respectively. We denote ${\sigma[\log(e^{(W^Tx)_{{y_P}}})-\log(e^{(W^Tx)_{{y_L}}}]}$ as ${\gamma({x}, {y_L, y_P})}$.

% \textbf{Statement:} Given a single layer pre-trained neural network, optimizing the weights using DPO results in formation of clusters of safe and unsafe samples in the output space and also results in decreased value of the lipschitz constant for unsafe inputs.
The gradient with respect to weight ${W}$ for the DPO objective is given by:
\begin{equation}
    {\Delta_W L(x,y_L,y_P)} = -{\Sigma_{x,y_P,y_L}\sigma[\log(e^{(W^Tx)_{y_P}})-\log(e^{(W^Tx)_{y_L}}]}
    {[\Delta_W\log(e^{(W^Tx)_{y_P}})-\Delta_W\log(e^{(W^Tx)_{y_L}})]}
\end{equation}

\begin{equation}
    {\Delta_W L(x,y_L,y_P) = -\Sigma_{x,y_P,y_L}\gamma(x, y_P, y_L)([\mathbb{0,0,0},x,\mathbb{0},...]-[x,\mathbb{0,0,0},...])}
\end{equation}
where $\mathtt{[\mathbb{0,0,0},x,\mathbb{0},...]}$ is $\mathbb{R^{d\times k}}$
Therefore the gradient update for an unsafe sample $\mathtt{x_u} \in$ \bgdbox{red}{$\mathcal{P_U}$} is given by
\begin{equation}
\mathtt{W_t = W_{t-1} + [\alpha\gamma(x, y_P, y_L)x,\mathbb{0,0}.., \mathbb{0}] -[\mathbb{0}, ..., \mathbb{0}, \alpha\gamma(x, y_P, y_L)x, \mathbb{0},..., \mathbb{0}]}
\end{equation}
In case of $\mathtt{x_s} \in$ \bgdbox{green}{$\mathcal{P_S}$}, the gradient update is given by
\begin{equation}
\mathtt{W_t = W_{t-1} + [\mathbb{0}, ..., \mathbb{0}, \alpha\gamma(x, y_P, y_L)x, \mathbb{0},..., \mathbb{0}] - [\alpha\gamma(x, y_P, y_L)x, \mathbb{0}, \mathbb{0},.., \mathbb{0}]}
\end{equation}
Suppose the first p samples are unsafe and remaining t-p safe samples, then at time step t, the model will be given by
\begin{multline}
\label{eq:update}
    {W_t = W + \Sigma_{i=1}^p\alpha\gamma_ix_i[\mathbb{1},\mathbb{0,0,0,0},...] - \Sigma_{i=p+1}^t\alpha\gamma_ix_i[\mathbb{1},\mathbb{0,0,0,0},...]} - \\ {\Sigma_{i=1}^p\alpha\gamma_ix_i[\mathbb{0},\mathbb{1}(y_i==2),\mathbb{1}(y_i==3),..., \mathbb{1}(y_i==\mathbb{K})] +} \\ {\Sigma_{i=p+1}^t\alpha\gamma_ix_i[\mathbb{0},\mathbb{1}(y_i==2),\mathbb{1}(y_i==3),..., \mathbb{1}(y_i==\mathbb{K})]}
\end{multline}
where $\mathbb{1}, \mathbb{0} \in \mathbb{R^d}$ vectors with all rows having values 1 and 0 respectively.

If \bgdbox{green}{${x_i}$} and \bgdbox{green}{${x_j}$}, ${i \neq j}$ are safe samples, using the definition of global lipschitz constant in Eq~\ref{eq:lips} we get 
\begin{multline}
{{||f(\bgdbox{green}{$x_i$}) - f(\bgdbox{green}{$x_j$})||}=||W^T(\bgdbox{green}{$x_i$}-\bgdbox{green}{$x_j$}) + \alpha[(\gamma_j-\gamma_i)(\mathbb{1}, \mathbb{0,0}, ...)} - \\ {\gamma_j[\mathbb{0,0}, ...,\mathbb{1}, \mathbb{0}, ..., \mathbb{0}] + \gamma_i[\mathbb{0,0}, ...,\mathbb{1}, \mathbb{0}, ..., \mathbb{0}]||}
\end{multline}

If \bgdbox{red}{${x_i}$} and \bgdbox{red}{${x_j}$}, ${i \neq j}$ are unsafe, we get
\begin{multline}
{{||f(\bgdbox{red}{$x_i$}) - f(\bgdbox{red}{$x_j$})||}=||W^T(\bgdbox{red}{$x_i$}-\bgdbox{red}{$x_j$}) + \alpha[(\gamma_i-\gamma_j)(\mathbb{1}, \mathbb{0}, \mathbb{0}, ...)} - \\ {\gamma_i[\mathbb{0,0}, ...,\mathbb{1}, \mathbb{0}, ..., \mathbb{0}] + \gamma_j[\mathbb{0}, \mathbb{0}, ...,\mathbb{1}, \mathbb{0}, ..., \mathbb{0}]||}
\end{multline}
As discussed in {A2}, ${W[:,i]=\Sigma_{i=1}^l\delta_i x_{i, y_i}}$. This gives:
\begin{multline}
{{||f(\bgdbox{green}{$x_i$}) - f(\bgdbox{green}{$x_j$})||}=||\alpha(\gamma_j-\gamma_i)(\mathbb{1}, \mathbb{0,0}, ...)} - \\ {(\alpha\gamma_j+\delta_j)[\mathbb{0,0}, ...,\mathbb{1},  \mathbb{0}, ..., \mathbb{0}] + (\alpha\gamma_i+\delta_i)[\mathbb{0,0}, ...,\mathbb{1}, \mathbb{0}, ..., \mathbb{0}]||}
\end{multline}

\begin{multline}
{{||f(\bgdbox{red}{$x_i$}) - f(\bgdbox{red}{$x_j$})||}=||\alpha(\gamma_i-\gamma_j)(\mathbb{1}, \mathbb{0,0}, ...)} - \\ {(\alpha\gamma_i-\delta_i)[\mathbb{0,0}, ...,\mathbb{1}, \mathbb{0}, ..., \mathbb{0}] + (\alpha\gamma_j-\delta_j)[\mathbb{0,0}, ...,\mathbb{1}, \mathbb{0}, ..., \mathbb{0}]||}
\end{multline}
Thus maximum value is given by 
\begin{equation}
    {max_{x_i, x_j} {||f(\bgdbox{green}{$x_i$}) - f(\bgdbox{green}{$x_j$})||} =  max_{\gamma_i, \gamma_j,\delta_i, \delta_j}\sqrt{(\alpha(\gamma_i-\gamma_j))^2 + (\alpha\gamma_i+\delta_i)^2 + (\alpha\gamma_j+\delta_j)^2 }}
\end{equation}

\begin{equation}
    {max_{x_i, x_j} {||f(\bgdbox{red}{$x_i$}) - f(\bgdbox{red}{$x_j$})||} =  max_{\gamma_i, \gamma_j, \delta_i, \delta_j}\sqrt{(\alpha(\gamma_i-\gamma_j))^2 + (\alpha\gamma_i-\delta_i)^2 + (\alpha\gamma_j-\delta_j)^2 }}
\end{equation}
Therefore on using unsafe samples, the maximum value of lipschitzness constant can decrease for a suitable value of learning rate $\alpha$.

Further in case of unlearning, we have $\gamma_i=\gamma_j=1$, this gives:
\begin{equation}
        {max_{x_i, x_j} {||f(\bgdbox{red}{$x_i$}) - f(\bgdbox{red}{$x_j$})||} =   max_{\delta_i, \delta_j}\sqrt{(\alpha-\delta_i)^2 + (\alpha-\delta_j)^2 }}
\end{equation}
In case of supervised safety fine-tuning, this expression will be given by:
\begin{equation}
    {max_{x_i, x_j} {||f(\bgdbox{red}{$x_i$}) - f(\bgdbox{red}{$x_j$})||} =  max_{\delta_i, \delta_j}\sqrt{\alpha^2 + \delta_i^2 + (\alpha-\delta_j)^2 }}
\end{equation}
Thus we get
$\mathcal{L}(f_{\theta^{Unl}}) \leq \mathcal{L}({f_{\theta^{SSFT}}}) \leq \mathcal{L}({f_{\theta^{IT}}})$ for unsafe samples for some learning rate  $\alpha<\text{min}{\delta_j}$.

\end{proof}
On the other hand, for safe samples, we have $\mathcal{L}(f_{\theta^{Unl}}) \geq \mathcal{L}({f_{\theta^{SSFT}}}) \geq \mathcal{L}({f_{\theta^{IT}}})$. This is also observed in our empirical analysis about lipschitzness constant presented in the main paper.
